# Supplementary material for: Robust Neural Machine Translation for Clean and Noisy Speech Transcripts
Source: arXiv:1910.10238 source file (2019-10-22)
Supplement: Supplementary file 1 [file appendixA.tex]

\begin{table*}[t]
\small
\begin{tabular}{l|l}
Clean &  that means we all share a common ancestor, an evolutionary grandmother, who lived around six million years ago. \\
Noisy &  that means we all share a common ancestor \ul{on evolutionary} grandmother who lived around six million years ago. \\
Base NMT & Ci\`o significa che tutti condividiamo un antenato comune sulla nonna evolutiva che ha vissuto circa sei milioni di anni fa. \\
Robust NMT & Ci\`o significa che tutti condividiamo un antenato comune e una nonna evolutiva che \`e vissuta circa sei milioni di anni fa. \\\hline

Clean & and we in the West couldn't understand how anybody would do this, how much this would restrict freedom of speech. \\
Noisy & we in the \ul{West. I couldn 't} understand how anybody \ul{would do how much} this would restrict freedom of speech. \\
Base NMT & Noi occidentali. Non riuscivo a capire come chiunque avrebbe fatto quanto questo avrebbe limitato la libert\`a di parola. \\
Robust NMT & In Occidente non riuscivo a capire come chiunque avrebbe fatto, quanto questo avrebbe limitato la libert\`a di parola. \\
\end{tabular}
\caption{Two examples of in which Robust NMT was ranked better than Base NMT. In the first example, a misrecognizer prepoosition (an$\rightarrow$on) is recovered, while in the second Robust MT is not harmed by misplaced punctuation. }
\label{tab:ex1}
\end{table*}

\begin{table*}[t]
\small
\begin{tabular}{l|l}
Clean & serve food  at a soup kitchen. clean up a neighborhood park . be a mentor. \\
Noisy & Sir. food in a soup kitchen. clean up the neighborhood park, be a mentor. \\
Base NMT & Signore\underline{.} Cibo in una cucina per minestre. Ripulire il parco del quartiere, essere un mentore. \\
Robust NMT & Signore\underline{,} cibo in una cucina per minestre, pulire il parco del quartiere, essere un mentore. %\\\\\hline

Clean & and no , this isn 't Burning Man or San Francisco \underline{.} ladies and gentlemen , meet your cousins. \\
Noisy & no , this is it . burning man or San Francisco \underline{?} ladies and gentlemen , meet your cousins. \\
Base NMT & No , questo \`e tutto . Un uomo in fiamme o San Francisco \underline{?} Signore e signori , incontrate i %vostri cugini. \\
Robust NMT & No , questo \`e un uomo in fiamme a San Francisco \underline{.} Signore e signori, incontrate i vostri %cugini. \\\\\hline

%Clean & remember , it 's free; none of us are making any money on this thing. \\
Noisy & minutes free. none of us were making any money on this thing. \\ 
Base NMT & Pochi minuti gratis. Nessuno di noi faceva soldi su questa cosa. \\
Robust NMT & Nessuno di noi stava facendo soldi su questa cosa. \\
\end{tabular}
\caption{Three examples in which Robust and Base NMT ranked equally.}
\label{tab:ex2}
\end{table*}

%\section{Additional examples}
%Tables \ref{tab:ex1} and \ref{tab:ex2} show, respectively, two examples in which the robust system is ranked  best by %all three judges, and three examples where the two systems are ranked equally by all three judges. In none of the cases %the translation by the robust system is perfect, but we can observe that its outputs are not harmed by clearly misplaced punctuation and that a misrecognized  preposition (an$\rightarrow$on) is properly recovered. The second example in Table \ref{tab:ex1} and the second in Table \ref{tab:ex2} show that Base NMT translates according to (wrong) boundaries given by punctuation, while Robust NMT consider a larger context, as punctuation is not given. This is particularly clear when it translates {\em uomo in fiamme \underline{a} San Francisco}, where ``a'' would translate ``in'' and not ``or''.  Also the third example in Table \ref{tab:ex2} shows that Robust NMT does not translate a part of the sentence not linked to the rest.
